# Supplementary material for: Model-tuning Via Prompts Makes NLP Models Adversarially Robust
Source: arXiv:2303.07320 source file (2023-12-06)
Supplement: Supplementary file 1 [file appendix.tex]

\section{Proof of Proposition~\ref{prop:resampling}}
\label{app:gumbel}
\begin{proof}
By assumption, we have importance weights $w_i$ that are proportional to the true importance weights, so that $w_i = C\frac{\pfeat(z_i)}{\qfeat(z_i)}$ for the $i$-th source example for some constant $C > 0$.
First suppose that $k=1$. Then,
\begin{align}
    \text{Prob. of sampling an example with feature value $z$} &= \frac{\sum_{i=1}^N \indicator[z_i = z] w_i}{\sum_{j=1}^N w_j}\\
    &= \frac{C\sum_{i=1}^N \indicator[z_i=z]\frac{\pfeat(z_i)}{\qfeat(z_i)}}{\sum_{j=1}^N C\frac{\pfeat(z_j)}{\qfeat(z_j)}}\\
    &= \frac{\frac{1}{N}\sum_{i=1}^N \indicator[z_i=z]\frac{\pfeat(z_i)}{\qfeat(z_i)}}{\frac{1}{N}\sum_{j=1}^N \frac{\pfeat(z_j)}{\qfeat(z_j)}}.
\end{align}

For $k\geq1$, we can similarly compute the probability of sampling the $m$-th example ($m \in \{1,\dots,k\}$) as:
\begin{align}
 \text{Prob. of sampling $m$-th example with feature value $z$} &= \frac{\frac{1}{N-m+1}\sum_{i=1}^{N-m+1} \indicator[z_i=z]\frac{\pfeat(z_i)}{\qfeat(z_i)}}{\frac{1}{N-m+1}\sum_{j=1}^{N-m+1} \frac{\pfeat(z_j)}{\qfeat(z_j)}},
\end{align}
where for notational convenience, we re-index the raw examples after selecting each example.

For each $m\in \{1,\dots,k\}$, the numerator converges to $\pfeat(z)$ as $N\rightarrow \infty$:
\begin{align}
   \frac{1}{N-m+1}\sum_{i=1}^{N-m+1} \indicator[z_i=z]\frac{\pfeat(z_i)}{\qfeat(z_i)} &= 
   \frac{1}{N-m+1}\sum_{i=1}^{N-m+1} \indicator[z_i=z]\frac{\pfeat(z)}{\qfeat(z)} \rightarrow \qfeat(z)\frac{\pfeat(z)}{\qfeat(z)} = \pfeat(z)
\end{align}
since $z_j$ (raw features) are sampled from $\qfeat$ (raw feature distribution).
For the same reason, the denominator converges to 1:
\begin{align}
   \frac{1}{N-m+1}\sum_{j=1}^{N-m+1} \frac{\pfeat(z_j)}{\qfeat(z_j)} \rightarrow \E_{\qfeat}\left[\frac{\pfeat(z_j)}{\qfeat(z_j)}\right] = 1.
\end{align}
Therefore the features of the $m$-th example is sampled from $\pfeat$ for all $m \in \{1,\dots,k\}$.
\end{proof}

\begin{figure}
\centering
\begin{subfigure}{0.33\textwidth}
\centering
\includegraphics[width=\textwidth]{figures/Random_retrieved_hist.pdf}
\end{subfigure}
\hfill
\begin{subfigure}{0.33\textwidth}
\centering
\includegraphics[width=\textwidth]{figures/Heuristic_classification_retrieved_hist.pdf}
\end{subfigure}
\hfill
\begin{subfigure}{0.33\textwidth}
\centering
\includegraphics[width=\textwidth]{figures/DSIR_retrieved_hist.pdf}
\end{subfigure}
\caption{Distribution of Pile data sources for datasets selected by \textbf{Left:} Random selection \textbf{Middle:} Heuristic classification and \textbf{Right:} \IS. Heuristic classification and \IS were restricted to select only 4\% of its dataset from Wikipedia, Books3, BookCorpus2, and Gutenberg.}
\label{fig:formal-text-dists}
\end{figure}

\section{Distribution of data sources for general-domain training}
\label{app:scratch-dists}
Figure~\ref{fig:formal-text-dists} shows the distribution of data sources (ArXiv, GitHub, News, etc.) from The Pile that were selected by random selection, heuristic classification, and \IS.
Heuristic classification and \IS aim to select formal text that are similar to text from Wikipedia or books.
Note that we restricted heuristic classification and \IS to select from data sources outside of Wikipedia and books sources (Books3, BookCorpus2, Gutenberg) for 96\% of the dataset, while 2\% is randomly selected from Wikipedia and the remaining 2\% are selected from the 3 book sources.
\IS seems to focus mostly selecting formal text from web data such as Pile-CC (which can still be quite varied), while the other methods select from a variety of sources.

\begin{figure}
\centering
\begin{subfigure}{0.24\textwidth}
\centering
\includegraphics[width=\textwidth]{figures/citation_intent_retrieved_hist.pdf}
\end{subfigure}
\hfill
\begin{subfigure}{0.24\textwidth}
\centering
\includegraphics[width=\textwidth]{figures/chemprot_retrieved_hist.pdf}
\end{subfigure}
\hfill
\begin{subfigure}{0.24\textwidth}
\centering
\includegraphics[width=\textwidth]{figures/hyperpartisan_retrieved_hist.pdf}
\end{subfigure}
\hfill
\begin{subfigure}{0.24\textwidth}
\centering
\includegraphics[width=\textwidth]{figures/helpfulness_retrieved_hist.pdf}
\end{subfigure}
\hfill
\begin{subfigure}{0.24\textwidth}
\centering
\includegraphics[width=\textwidth]{figures/sciie_retrieved_hist.pdf}
\end{subfigure}
\hfill
\begin{subfigure}{0.24\textwidth}
\centering
\includegraphics[width=\textwidth]{figures/rct_retrieved_hist.pdf}
\end{subfigure}
\hfill
\begin{subfigure}{0.24\textwidth}
\centering
\includegraphics[width=\textwidth]{figures/ag_news_retrieved_hist.pdf}
\end{subfigure}
\hfill
\begin{subfigure}{0.24\textwidth}
\centering
\includegraphics[width=\textwidth]{figures/imdb_retrieved_hist.pdf}
\end{subfigure}
\caption{Distribution of Pile data sources selected by \IS for different target distributions. The four columns from left to right represent 4 domains: CS papers, Biomedical text, News, and Reviews.}
\label{fig:continued-pretrain-dists}
\end{figure}

\section{Distribution of data sources for continued pretraining}
\label{app:continued-dists}
Figure~\ref{fig:continued-pretrain-dists} shows the distribution of Pile data sources selected by \IS for different target distributions. 
Each of the 4 columns represents a domain: CS papers, Biomedical text, News, and Reviews. The distribution of data sources for target distributions from the same domain are similar. When the target is a task from the CS domain, the distribution of data sources is the most diverse. Biomedical and news domains are particularly different; when the target is from the biomedical domain, most of the selected examples are from PubMed Abstracts and PubMed Central, and when the target is from the news domain, most of the selected examples are from web data (Pile-CC and OpenWebText2).

\begin{table}[t]
\centering
\caption{Continued pretraining results on the GLUE dev set when the target distribution is formal text. \IS improves average GLUE performance by 0.4--0.7\% over all baselines. All fine-tuning results are averaged over 5 seeds. Following RoBERTa~\citep{liu2019roberta}, for RTE, STS, and MRPC we fine-tune starting from the MNLI model instead of from scratch.}
\begin{adjustbox}{max width=\textwidth}
\begin{tabular}{lrrrrrrrrr}
\toprule
 & MNLI  & QNLI  & QQP   & RTE   & SST-2 & MRPC  & CoLA  & STS-B & Avg      \\ \midrule
BERT-base (no continued pretrain)                & 84.29$_{0.41}$ & 91.26$_{0.16}$ & 90.23$_{0.06}$ & 76.39$_{3.80}$ & 92.34$_{0.34}$ & 86.42$_{2.49}$ & 56.36$_{1.49}$ & 90.11$_{0.23}$ & 83.43   \\
Random selection         & 83.82$_{0.48}$ & 89.86$_{0.63}$ & 90.47$_{0.39}$ & 76.03$_{2.20}$                         & 92.00$_{0.31}$    & 87.21$_{1.47}$ & 59.00$_{2.57}$    & 90.32$_{0.17}$ & 83.59 \\
Heuristic classification & 84.03$_{0.33}$ & 90.47$_{0.65}$ & 90.46$_{0.36}$ & 76.75$_{1.74}$ & 91.88$_{0.42}$ & 86.03$_{0.78}$ & 56.03$_{4.22}$ & 90.30$_{0.22}$  & 83.24 \\
\IS & 84.21$_{0.47}$ & 90.78$_{0.42}$ & 90.45$_{0.39}$ & 78.34$_{1.75}$ & 92.09$_{0.59}$ & 87.16$_{0.77}$ & 58.41$_{5.86}$ & 90.49$_{0.19}$ & \textbf{83.99} \\
\bottomrule
\end{tabular}
\end{adjustbox}
\end{table}

\section{Continued pretraining results when target is formal text}
\label{app:continued-formal}
We also consider using the same datasets for continued pretraining, starting from the public BERT-base checkpoint.
Here, all data selection methods improve over BERT-base on the GLUE dev set.
Similarly to training from scratch, we find that heuristic classification slightly decreases performance compared to random selection (by 0.2\% on average). 
\IS improves over random selection by 0.4\% and over BERT-base by 0.6\%, achieving almost 84\% on the GLUE dev set.

\section{Data selection details}
\label{app:data-details}
\paragraph{Data preprocessing.}
We select data from The Pile~\citep{gao2020pile}, which comes in 30 random chunks. We reserve chunk 0 for validation purposes and only consider the last 29 chunks.
We first divided the documents in The Pile into chunks of 128 ``words'', according to whitespace tokenization.
These chunks define the examples that we do data selection on, totaling 1.7B examples.
For heuristic classification and \IS, we first apply a manual quality filter (Appendix~\ref{app:quality-filter}) and only consider the examples that pass the filter.
Random selection selects from the unfiltered Pile.

\paragraph{Heuristic classification.}
We use a bigram fasttext classification model~\citep{joulin2017bag}, which first forms a list of unigrams and bigrams, hashes them into a predefined number of tokens (2M in this case), maps these tokens into learned feature vectors, and then learns a logistic regression model on top of averaged feature vectors across the model.
We initialize the feature vectors from 300 dimensional pretrained subword fasttext vectors trained from Common Crawl.
We use the fasttext hyperparameter autotuning functionality with a duration timeout of 30 minutes.

The classification model is trained on a balanced dataset of examples from The Pile validation set and examples from the target distribution (downstream unlabeled training inputs or Wikipedia/book text from The Pile validation set). We downsample the larger dataset of the two to create the balanced dataset. Each example is lowercased and stripped of newlines by first tokenizing using the NLTK word tokenizer and rejoining the words with spaces.

For noisy thresholding, we select a raw example with probability $\rho_i$ predicted by the fasttext model if $\rho_i > 1- \beta_i$, where $\beta_i$ is sampled from a Pareto distribution with shape parameter 9. If the number of examples that do not cross the threshold is smaller than the desired number of examples $k$, then we repeat this process on the examples that were not chosen and continue to add to the dataset. After we have chosen at least $k$ examples, we take $k$ random samples without replacement from the chosen examples.

For top-$k$ heuristic classification, we simply take the examples with the top-$k$ predicted probabilities $\rho_i$.

\paragraph{Importance resampling.}
Our importance resampling-based methods use a bag-of-words generative model of text.
We process each example by lowercasing and splitting into words using the WordPunct tokenizer from NLTK~\citep{bird2009nltk}.
Following~\citep{joulin2017bag}, we incorporate unigram and bigram information by hashing the unigrams and bigrams into 10k buckets, which defines a vocabulary of 10k ``words'' for the generative model.
Both unigrams and bigrams are hashed into the same space of words.
We learn two bag-of-words models, one for the target and one for The Pile, using target data (downstream unlabeled training inputs or Wikipedia/book text from The Pile validation set) and Pile validation data.
The parameters of the models are learned by simply counting the word frequencies across the dataset.

For unigram-based \IS, we use the RoBERTa tokenizer~\citep{devlin2019bert}, which allows us to avoid hashing. With bigrams, this is more difficult since we must consider $50000^2$ pairs of tokens in the RoBERTa vocabulary. Still, even in the unigram case we find that there are often tokens that are never seen in the target dataset, so we smooth the MLE parameters by mixing with the uniform distribution over tokens with a weight of 1e-5.

\paragraph{Implementation of importance resampling.}
We implement importance resampling with the Gumbel top-$k$ trick~\citep{vieira2014gumbel,kim2016exact,xie2019subset,kool2019stochastic}, which produces $k$ samples without replacement according to the softmax distribution of the given scores.
In the Gumbel top-$k$ procedure, we add IID standard Gumbel noise $g_i$ to each log-importance weight to produce a score $s_i = \log\frac{\hatpfeat(z_i)}{\hatqfeat(z_i)} + g_i$ for each raw example. We select the examples corresponding to the top $k$ scores.
Note that producing the log-likelihood ratios and adding independent Gumbel noise to them can be trivially parallelized, and selecting top $k$ can be done in linear time with the introselect algorithm~\citep{musser1999introspective}, implemented by \texttt{numpy.argpartition}.

\begin{table}[tbp]
\caption{Hyperparameters for training general-domain LMs from scratch. }
\label{tab:general-scratch-hyperparams}
\centering
\begin{tabular}{lr}
\toprule
Architecture & BERT-base\\
Max token length & 128\\
Batch size & 4096 \\
Learning rate & 1e-3 or 8e-4\\
Learning rate schedule & Linear \\
Weight decay & 0.01\\
Warmup steps & 3000\\
Total steps & 50000\\
Optimizer & AdamW\\
Adam $\beta_1$ & 0.9\\
Adam $\beta_2$ & 0.999\\
Adam $\epsilon$ & 1e-8\\
GPUs & 4 Titan RTX\\
\bottomrule
\end{tabular}
\end{table}
\begin{table}[tbp]
\caption{Hyperparameters for continued pretraining of general-domain LMs. }
\label{tab:continued-general-hyperparams}
\centering
\begin{tabular}{lr}
\toprule
Architecture & BERT-base\\
Max token length & 512\\
Batch size & 2048 \\
Learning rate & 1e-4\\
Learning rate schedule & Linear \\
Weight decay & 0.01\\
Warmup steps & 1440\\
Total steps & 25000\\
Optimizer & AdamW\\
Adam $\beta_1$ & 0.9\\
Adam $\beta_2$ & 0.999\\
Adam $\epsilon$ & 1e-8\\
GPUs & 4 Titan RTX\\
\bottomrule
\end{tabular}
\end{table}

\paragraph{Sampling data for general-domain LMs.}
To select a dataset that is suitable for both pretraining from scratch at token length 128 and continued pretraining with token length 512, we choose to first select 102.4M examples then concatenate every two examples to create 51.2M examples.
This ensures that the examples are long enough for a max token length of 512 without much padding.
We train the importance weight estimator or fasttext classifier from The Pile validation set, where the target is Wikipedia + BookCorpus2 + Gutenberg + Books3 and the raw data come from the rest of the data sources in The Pile.
We first select 98.4M examples from non-Wikipedia and book data, then randomly select 2M from Wikipedia and 0.66M each from BookCorpus2, Gutenberg, and Books3. We mix in some examples from Wikipedia and books to balance the distribution of sources and to reduce catastrophic forgetting in continued pretraining. After this, we concatenate every two examples.

\paragraph{Details for ablations.}
We ablate top-$k$ heuristic classification in Section~\ref{sec:continued} in two ways.
First, we consider the original heuristic classification method, which takes classifier probabilities $\rho_i=f(x_i)$ for an example and selects the example if $\rho_i > 1-\beta_i$ where $\beta_i$ is a Pareto random variable.
Second, we consider heuristic classification with importance resampling by first calibrating the classifier's probabilities with Platt scaling~\citep{platt1999probabilistic} against a validation set, then using the calibrated probabilities $\rho_i$ to compute the importance weight $\log\frac{\rho_i}{1-\rho_i}$. Similarly to \IS, we use the Gumbel top-$k$ trick to select a subset using these importance weights.

We ablate the \IS approach by replacing the generative importance weight estimator with a discriminative one.
We use the same hashing method and define the features as 10k-dimensional counts of the n-grams. We normalize each count vector to sum to 1.
On top of these features, we train a logistic regression classifier using the same dataset used to train the fasttext classifier in heuristic classification.
We tune an L2 regularization weight based on best held-out accuracy (we further split the validation set in half to create another held out set) in the binary classification task.
Similarly as above, we calibrate the probabilities using Platt scaling and use the classifier probabilities to compute the importance weight.

\section{Training details for training general-domain LMs}
\label{app:training-scratch}
\paragraph{Pretraining from scratch.}
Table~\ref{tab:general-scratch-hyperparams} shows the hyperparameters for training general-domain LMs from scratch. For all models except \IS, we use learning rate 1e-3. We use 8e-4 for \IS since we found that 1e-3 leads to divergence in the training. We use 16 accumulation steps with 4 GPUs to achieve a large batch size of 4096, following~\citet{izsak2021how}.
Our hyperparameters result in a compute budget of 26B tokens processed (128 $\times$ 4096 $\times$ 50000).
Each training run takes about 50 hours.
Our pretraining implementation is adapted from~\citet{yao2022scratch}.

\paragraph{Continued pretraining (Appendix~\ref{app:continued-formal}).}
Table~\ref{tab:continued-general-hyperparams} shows the hyperparameters for continued pretraining general-domain LMs. We continue pretraining from the BERT-base~\citep{devlin2019bert} checkpoint. During BERT training, they process 43B tokens. We process 26B tokens during training so that the total compute after continued pretraining is 69B tokens. Each continued pretraining run takes about 60 hours.

\paragraph{Fine-tuning on GLUE.}
We follow the hyperparameters used by RoBERTa~\citep{liu2019roberta} for fine-tuning on GLUE (Tables~\ref{tab:finetune-general-hyperparams} and~\ref{tab:shared-finetune-general-hyperparams}).
While RoBERTa searches over a space of hyperparameters, we just use the hyperparameters set for each task from the RoBERTa code base.
The fine-tuning for RTE, MRPC, and STSB continues from the fine-tuned model for MNLI, following~\citet{liu2019roberta}.
We use the default HuggingFace code for GLUE fine-tuning.

\begin{table}[tbp]
\caption{Dataset-specific hyperparameters for fine-tuning LMs on GLUE, following best hyperparameters from RoBERTa~\citep{liu2019roberta}.}
\label{tab:finetune-general-hyperparams}
\centering
\begin{tabular}{lrrrr}
\toprule
& Epochs & Batch size & Learning rate & Continue from MNLI?\\
MNLI & 10 & 32 & 1e-5 & N\\
RTE & 10 & 16 & 2e-5 & Y\\
MRPC & 10 & 16 & 1e-5 & Y\\
STSB & 10 & 16 & 2e-5 & Y\\
COLA & 10 & 16 & 1e-5 & N\\
QQP & 10 & 32 & 1e-5 & N\\
SST2 & 10 & 32 & 1e-5 & N\\
QNLI & 10 & 32 & 1e-5 & N\\
\bottomrule
\end{tabular}
\end{table}
\begin{table}[tbp]
\caption{Shared hyperparameters for fine-tuning LMs on GLUE, following~\citet{liu2019roberta}.}
\label{tab:shared-finetune-general-hyperparams}
\centering
\begin{tabular}{lr}
\toprule
Architecture & BERT-base\\
Max length & 128 (from scratch) or 512 (continued pretrain)\\
Weight decay & 0.1\\
Optimizer & AdamW\\
Adam $\beta_1$ & 0.9\\
Adam $\beta_2$ & 0.98\\
Adam $\epsilon$ & 1e-6\\
Warmup ratio & 0.06\\
LR schedule & Polynomial\\
Precision & FP16\\
GPUs & 1 Titan RTX\\
\bottomrule
\end{tabular}
\end{table}
\section{Training details for continued pretraining of domain-specific LMs}
\label{app:training-continued}
\paragraph{Pretraining.}
Table~\ref{tab:continued-pretrain-hyperparams} shows the hyperparameters for continued pretraining domain-specific LMs. We choose the pretraining compute budget to equal the number of tokens processed in the DAPT models from~\citet{gururangan2020don}. For all models, we first try pretraining with learning rate 5e-4, and if training diverges, we use 1e-4.

\paragraph{Fine-tuning.}
Table~\ref{tab:continued-finetune-hyperparams} shows the hyperparameters for fine-tuning on domain-specific datasets. We use the fine-tuning code from~\citet{gururangan2020don} and follow their fine-tuning protocols. For datasets from CS/Biomed/News domains, we use a max token length of 256 to match the pretraining length.
For Reviews (IMDB and Helpfulness) datasets, we use a max token length of 512 since this seems to change performance significantly.
For DAPT models~\citep{gururangan2020don}, we use a max token length of 512 for all datasets, which matches their protocol.
Following~\citet{gururangan2020don}, we choose either 3 or 10 epochs based on average validation performance over 5 seeds.
Our fine-tuning implementation follows~\citet{gururangan2020don}.

\begin{table}[tbp]
\caption{Hyperparameters for continued pretraining on domain-specific data.}
\label{tab:continued-pretrain-hyperparams}
\centering
\begin{tabular}{lr}
\toprule
Architecture & RoBERTa-base\\
Max token length & 256\\
Total steps & 12500\\
Batch size & 4096\\
Weight decay & 0.01\\
Adam $\beta_1$ & 0.9\\
Adam $\beta_2$ & 0.999\\
Adam $\epsilon$ & 1e-8\\
Warmup steps & 720\\
LR schedule & Linear\\
Learning rate & 5e-4 or 1e-4\\
GPUs & 4 Titan RTX\\
\bottomrule
\end{tabular}
\end{table}
\begin{table}[tbp]
\caption{Hyperparameters for fine-tuning on domain-specific data.}
\label{tab:continued-finetune-hyperparams}
\centering
\begin{tabular}{lr}
\toprule
Architecture & RoBERTa-base\\
Max token length & 256 or 512\\
Epochs & 3 or 10\\
Patience & 3 epochs\\
Batch size & 4096\\
Weight decay & 0.1\\
Optimizer & AdamW\\
Adam $\beta_1$ & 0.9\\
Adam $\beta_2$ & 0.98\\
Adam $\epsilon$ & 1e-6\\
Warmup ratio & 0.06\\
LR schedule & Linear\\
GPUs & 1 Titan RTX\\
\bottomrule
\end{tabular}
\end{table}

\section{Computing the KL reduction metric}
\label{app:correlation}
To compute the KL reduction metric for a particular dataset, we took the first 100k examples from the dataset and computed the hashed n-gram counts.
Normalizing these counts gives an MLE estimate of the hashed n-gram distribution for the dataset.
We use the same procedure to compute the hashed n-gram distribution parameters for The Pile (from the Pile validation set).

For manual curation (DAPT), we attempted to download the datasets used in the paper (RealNews~\citep{zellers2019neuralfakenews}, S2ORC~\citep{lo2020s2orc}, and Amazon reviews~\citep{he2016amazonreview}). However, ~\citet{gururangan2020don} uses an internal version of S2ORC that cannot be released. We approximate S2ORC for CS papers and Biomed by using the first 100k documents in the public version of S2ORC that contain `Computer Science' and `Medicine' as a metadata field, respectively.

For RoBERTa, we approximate the pretraining distribution by computing the hashed n-gram distribution from Wikipedia and books data in the Pile validation set.

\section{Quality filter}
\label{app:quality-filter}
For heuristic classification and IS methods, we devise a few hand-crafted ways to filter out low quality data as a preprocessing step, according to
\begin{itemize}
\item Word length: between 40 and 500
\item Repeat ratio, defined as $\max_{\text{word}}\frac{\text{\# occurrences of word in example}}{\text{example word length}}$: between 0.02 and 0.2
\item Informativeness ratio, defined as $\frac{\text{\# of non-stopwords and non-punctuation in example}}{\text{example word length}}$: between 0.3 and 0.7
\item Numeric ratio, defined as $\frac{\text{\# of numbers in example}}{\text{example word length}}$: less than 0.2
\end{itemize}
The words are based on the NLTK word tokenizer~\citep{bird2009nltk}. These are difficult for a simple n-gram based importance weight estimator or classifier to use as features because it requires global context.
We decide to keep vs. discard examples using some simple thresholds on the above values, decided using inspection on the Pile validation set.
Below, we detail some statistics of the quality filtering procedure and provide some data examples.

\paragraph{Statistics of quality filtering.}
With the above thresholds, we find that:
\begin{itemize}
\item The length filter is the most selective --- after applying the length filter, only 55\% of the examples are left.
\item The repeat ratio filter keeps 78\% of the data.
\item The informativeness filter keeps 72\% of the data.
\item The numeric filter keeps 91\% of the data.
\item Overall, when applying all the filters at the same time, 52\% of the examples are kept. Thus, we are mainly filtering by length, which seems like a good proxy for quality.
\end{itemize}

\paragraph{Kept vs. discarded examples according to quality filter.}

First, we show the beginning characters from some randomly selected kept vs. discarded examples.
\begin{small}
\begin{verbatim}
KEPT:
all rights, the girl should be hanged for coining and thievery, and you, sir,
millennia of ancient carvings, magical swords and glittering jewels and textiles.
Kmax, and mean asphericity ( Q) on corneal tomography were evaluated
[M]other selects a therapist who requires co-pay in\n
informations about call once you are done and you don't need info anymore
\end{verbatim}

\begin{verbatim}
DISCARDED:
                                                    (31)\\\n
SUCH DAMAGE.\n#################################################################
            +                          1                                       
           "mpls"\n        ],\n        "setup": [\n            [\n             
   1993--1997, 48 months                         NA (\\<5 yr age)              
  var value = formattedTime + '\\t' + type + '\\t' + name + '\\t' + eventTxt +
                                                              FILED\n         
110.88 (108.42 to 113.34)   107.89 (105.28 to 110.50)   1.25 (-2.18 to 4.67) 
Wye Mun no podia evitar recordar lo que su padre siempre decia: <<Nunca olvides
               2.18                                                           
bG9hdDpsZWZ0O21hcmdpbjoycHggNXB4OyB0ZXh0LWFsaWduOmNlbnRlcjsiPjxhIGhyZWY9Imh0\n
\end{verbatim}
\end{small}

\paragraph{Extreme length examples.}
Very short examples tend to be data snippets or otherwise nonsensical:
\begin{small}
\begin{verbatim}
278713.303 3771574.556 by arc centered at 280828.793 3766437.062 94a to 
279188.184 3771745.314 by arc centered at 280945.177 3766474.440 to 280325.491 
3771995.774 by arc centered at 281478.555 3766560.741 to
\end{verbatim}
\end{small}
Very long examples tend to be dense code, repetitive, or very technical:

\begin{tiny}
\begin{verbatim}
$ y ' = \cap_ { h \in \mathcal { d } ( y ) \setminus g. \ { h_0 \ } } h^+ $ . the cube complex $ v = h_0^- \cap y ' $ is called a * vertebra * .
see figures \ [ fig : pentagons\ ] and \ [ vertebra\ ] . ( -4.37 , -3.17 ) rectangle ( 6.57,5.42 ) ; ( 0,0 ) – ( 0,1 ) ;
( 0,0 ) – ( 1,0 ) ; ( 1,1 ) – ( 1,0 ) ; ( 1,1 ) – ( 1,1.56 ) ; ( 0.71,1.71 ) – ( 0.85,1.71 ) ; plot\ [ domain=3.93:4.71 ,
variable=\ ] ( [ 1\ * 0.71\ * cos ( r ) +0\ * 0.71\ * sin ( r ) ] { } , [ 0\ * 0.71\ * cos ( r ) +1\ * 0.71\ * sin ( r ) ] { } ) ; 
plot\ [ domain=4.71:5.5 , variable=\ ] ( [ 1\ * 0.71\ * cos ( r ) +0\ * 0.71\ * sin ( r ) ] { } , [ 0\ * 0.71\ * cos ( r ) +1\ * 0.71\ 
* sin ( r ) ] { } ) ; plot\ [ domain=-0.79:0 , variable=\ ] ( [ 1\ * 0.71\ * cos ( r ) +0\ * 0.71\ * sin ( r ) ] { } , [ 0\ * 0.71\ 
* cos ( r ) +1\ * 
0.71\ * sin ( r ) ] { } ) ; plot\ [ domain=3.142:4.71 , variable=\ ] ( [ 1\ * 0.15\ * cos ( r ) +0\ * 0.15\ * sin ( r ) ] { } , 
[ 0\ * 0.15\ * cos ( r ) +1\ * 0.15\ * sin ( r ) ] { } ) ; plot\ [ domain=3.93:4.71 , variable=\ ] ( [ -1\ * 0.71\ * cos ( r ) 
+0\ * 0.71\ * sin ( r ) ] { } , [ 0\ * 0.71\ * cos ( r ) +1\ * 0.71\ * sin ( r ) ] { } ) ; plot\ [ domain=4.71:5.5 , 
variable=\ ] ( [ -1\ * 0.71\ * cos ( r ) +0\ * 0.71\ * sin ( r ) ] { } , [ 0\ * 0.71\ * cos ( r ) +1\ * 0.71\ * sin ( r ) ] { } ) ; 
plot\ [ domain=-0.79:0 , variable=\ ] ( [ -1\ * 0.71\ * cos ( r ) +0\ * 0.71\ * sin ( r ) ] { } , [ 0\ * 0.71\ * cos ( r ) +1\ * 
0.71\ * sin ( r ) ] { } ) ; plot\ [ domain=3.142:4.71 , variable=\ ] ( [ -1\ * 0.15\ * cos ( r ) +0\ * 0.15\ * sin ( r ) ] { } , 
[ 0\ * 0.15\ * cos ( r ) +1\ * 0.15\ * sin ( r ) ] { } ) ; ( 2,0 ) – ( 2,1 ) ; ( 2,0 ) – ( 1,0 ) ; ( 1,1 ) – ( 1,1.56 ) ; 
( 1.29,1.71 ) – ( 1.15,1.71 ) ; plot\ [ domain=3.93:4.71 , variable=\ ] ( [ -1\ * 0.71\ * cos ( r ) +0\ * 0.71\ * sin ( r ) ] { } , 
[ 0\ * 0.71\ * cos ( r ) +1\ * 0.71\ * sin ( r ) ] { } ) ; plot\ [ domain=4.71:5.5 , variable=\ ] ( [ -1\ * 0.71\ * cos ( r ) +0\ * 
0.71\ * sin ( r ) ] { } , [ 0\ * 0.71\ * cos ( r ) +1\ * 0.71\ * sin ( r ) ] { } ) ; plot\ [ domain=-0.79:0 , variable=\ ] ( [ -1\ 
* 0.71\ * cos ( r ) +0\ * 0.71\ * sin ( r ) ] { } , [ 0\ * 0.71\ * cos ( r ) +1\ * 0.71\ * sin ( r ) ] { } ) ; plot\ [ 
domain=3.142:4.71 , variable=\ ] ( [ -1\ * 0.15\ * cos ( r ) +0\ * 0.15\ * sin ( r ) ] { } , [ 0\ * 0.15\ * cos ( r ) +1\ * 0.15\ 
* sin ( r ) ] { } ) ; plot\ [ domain=3.93:4.71 , variable=\ ] ( [ 1\ * 0.71\ * cos ( r ) +0\ * 0.71\ * sin ( r ) ] { } , 
[ 0\ * 0.71\ * cos ( r ) +1\ * 0.71\ * sin ( r ) ] { } ) ; plot\ [ domain=4.71:5.5 , variable=\ ] ( [ 1\ * 0.71\ * cos ( r ) 
+0\ * 0.71\ * sin ( r ) ] { } , [ 0\ * 0.71\ * cos ( r ) +1\ * 0.71\ * sin ( r ) ] { } ) ; plot\ [ domain=-0.79:0 , variable=\ ] 
( [ 1\ * 0.71\ * cos ( r ) +0\ * 0.71\ * sin ( r ) ] { } , [ 0\ * 0.71\ * cos ( r ) +1\ * 0.71\ * sin ( r ) ] { } ) ; plot\ 
[ domain=3.142:4.71 , variable=\ ] ( [ 1\ * 0.15\ * cos ( r ) +0\ * 0.15\ * sin ( r ) ] { } , [ 0\ * 0.15\ * cos ( r ) +
1\ * 0.15\ * sin ( r ) ] { } ) ; ( 4,0 ) – ( 4,1 ) ; ( 4,0 ) – ( 3,0 ) ; ( 3,1 ) – ( 3,0 ) ; ( 3,1 ) – ( 3,1.56 ) ; ( 3.29,1.71 ) 
– ( 3.15,1.71 ) ; ( 2,0 ) – ( 3,0 ) ; ( 3,1 ) – ( 3,1.56 ) ; ( 2.71,1.71 ) – ( 2.85,1.71 ) ; plot\ [ domain=3.93:4.71 ,
variable=\ ] ( [ -1\ * 0.71\ * cos ( r ) +0\ * 0.71\ * sin ( r ) ] { } , [ 0\ * 0.71\ * cos ( r ) +1\ * 0.71\ * sin ( r ) ] { } ) ;
plot\ [ domain=4.71:5.5 , variable=\ ] ( [ -1\ * 0.71\ * cos ( r ) +0\ * 0.71\ * sin ( r ) ] { } , [ 0\ * 0.71\ * cos ( r ) +1\ * 
0.71\ * sin ( r ) ] { } ) ; plot\ [ domain=-0.79:0 , variable=\ ] ( [ -1\ * 0.71\ * cos ( r ) +0\ * 0.71\ * sin ( r ) ] { } , 
[ 0\ * 0.71\ * cos ( r ) +1\ * 0.71\ * sin ( r ) ] { } ) ; plot\ [ domain=3.142:4.71 , variable=\ ] ( [ -1\ * 0.15\ * 
cos ( r ) +0\ * 0.15\ * sin ( r ) ] { } , [ 0\ * 0.15\ * cos ( r ) +1\ * 0.15\ * sin ( r ) ] { } ) ; plot\ [ domain=3.93:4.71 , 
variable=\ ] ( [ 1\ * 0.71\ * cos ( r ) +0\ * 0.71\ * sin ( r ) ] { } , [ 0\ * 0.71\ * cos ( r ) +1\ * 0.71\ * sin ( r ) ] { } ) ;
plot\ [ domain=4.71:5.5 , variable=\ ] ( [ 1\ * 0.71\ * cos ( r ) +0\ * 0.71\ * sin ( r ) ] { } , [ 0\ * 0.71\ * cos ( r ) +1\ * 
0.71\ * sin ( r ) ] { } ) ; plot\ [ domain=-0.79:0 , variable=\ ] ( [ 1\ * 0.71\ * cos ( r ) +0\ * 0.71\ * sin ( r ) ] { } , 
[ 0\ * 0.71\ * cos ( r ) +1\ * 0.71\ * sin ( r ) ] { } ) ; plot\ [ domain=3.142:4.71 , variable=\ ] ( [ 1\ * 0.15\ * cos ( r ) +
0\ * 0.15\ * sin ( r ) ] { } , [ 0\ * 0.15\ * cos ( r ) +1\ * 0.15\ * sin ( r ) ] { } ) ; plot\ [ domain=3.93:4.71 , 
variable=\ ] ( [ 1\ * 0.71\ * cos ( r ) +0\ * 0.71\ * sin ( r ) ] { } , [ 0\ * 0.71\ * cos ( r ) +1\ * 0.71\ * sin ( r ) ] { } ) ; 
plot\ [ domain=4.71:5.5 , variable=\ ] ( [ 1\ * 0.71\ * cos ( r ) +0\ * 0.71\ * sin ( r ) ] { } , [ 0\ * 0.71\ * cos ( r ) +1\ * 0.71\ * 
sin ( r ) ] { } ) ; plot\ [ domain=-0.79:0 , variable=\ ] ( [ 1\ * 0.71\ * cos ( r ) +0\ * 0.71\ * sin ( r ) ] { } , [ 0\ * 0.71\ * 
cos ( r ) +1\ * 0.71\ * sin ( r ) ] { } ) ; plot\ [ domain=3.142:4.71 , variable=\ ] ( [ 1\ * 0.15\ * cos ( r ) +0\ * 0.15\ * 
sin ( r ) ] { } , [ 0\ * 0.15\ * cos ( r ) +1\ * 0.15\ * sin ( r ) ] { } ) ; plot\ [ domain=3.93:4.71 , variable=\ ] 
( [ -1\ * 0.71\ * cos ( r ) +0\ * 0.71\ * sin ( r ) ] { } , [ 0\ * 0.71\ * cos ( r ) +1\ * 0.71\ * sin ( r ) ] { } ) ; 
plot\ [ domain=4.71:5.5 , variable=\ ] ( [ -1\ * 0.71\ * cos ( r ) +0\ * 0.71\ * sin ( r ) ] { } , [ 0\ * 0.71\ * cos ( r ) +
1\ * 0.71\ * sin ( r ) ] { } ) ; plot\ [ domain=-0.79:0 , variable=\ ] ( [ -1\ * 0.71\ * cos ( r ) +0\ * 0.71\ * sin ( r ) ] { } , 
[ 0\ * 0.71\ * cos ( r ) +1\ * 0.71\ * sin ( r ) ] { } ) ; plot\ [ domain=3.142:4.71 , variable=\ ] ( [ -1\ * 0.15\ * cos ( r ) 
+0\ * 0.15\ * sin ( r ) ] { } , [ 0\ * 0.15\ * cos ( r ) +1\ * 0.15\ * sin ( r ) ] { } ) ; ( 8,0 ) – ( 8,1 ) ; ( 8,0 ) – ( 7,0 ) ; 
( 7,1 ) – ( 7,0 ) ; ( 7,1 ) – ( 7,1.56 ) ; ( 7.29,1.71 ) – ( 7.15,1.71 ) ; ( 6,0 ) – ( 6,1 ) ; ( 6,0 ) – ( 7,0 ) ; ( 7,1 ) – 
( 7,1.56 ) ; ( 6.71,1.71 ) – ( 6.85,1.71 ) ; ( 4,0 ) – ( 5,0 ) ; ( 5,1 ) – ( 5,0 ) ; ( 5,1 ) – ( 5,1.56 ) ; ( 4.71,1.71 ) – 
( 4.85,1.71 ) ; ( 6,0 ) – ( 5,0 ) ; ( 5,1 ) – ( 5,1.56 ) ; ( 5.29,1.71 ) – ( 5.15,1.71 ) ; plot\ [ domain=3.93:4.71 
, variable=\ ] ( [ -1\ * 0.71\ * cos ( r ) +0\ * 0.71\ * sin ( r ) ] { } , [ 0\ * 0.71\ * cos ( r ) +1\ * 0.71\ * sin ( r ) ] { } ) ;
\end{verbatim}
\end{tiny}

\paragraph{Extreme repeat ratio example.} Examples with a high repeat ratio are mostly examples without much content except for one repeated token, sometimes within code:
\begin{small}
\begin{verbatim}
$ d_h ( x , y+\delta ) $ -- -- -- -- -- -- -- -- -- -- -- -- -- --
-- -- -- -- -- -- -- -- -- -- -- -- -- -- -- -- -- -- -- -- -- --
-- -- -- -- -- -- -- -- -- -- -- -- -- -- -- -- -- -- -- -- -- --
-- -- -- -- -- -- -- -- -- -- -- -- -- -- -- -- -- -- -- -- -- --
-- -- -- -- -- -- -- -- -- -- -- -- -- -- -- -- -- -- -- -- -- --
-- -- -- -- -- -- $ \left ( -\infty , \frac { 3\delta } { 4 } 
+\eps\delta\right ) $ $ ( x_0 , y ) $ –

-- -- -- -- -- -- -- -- -- -- -- -- -- -- -- -- -- -- -- -- -- --
-- -- -- -- -- -- -- -- -- -- -- -- -- -- -- -- -- -- -- -- -- --
-- -- -- -- -- -- -- -- -- -- -- -- -- -- -- -- -- -- -- -- -- --
-- -- - -- -- -- -- -- -- -- - -- -- -- -- -- -- -- - -- -- -- --
-- -- -- -- - -- -- -- -- -- -- -- -- - -- -- -- 
* * i look forward to one day becoming a mother * * * * 0 * * . 
* * 871 * * * * 0 * * . * * 870 * * -0.130 -0.312 0.066 -0.286
\end{verbatim}
\end{small}

\paragraph{Extreme informativeness ratio examples.}
Very low informative ratio examples also tend to be (sometimes extremely) short:
\begin{verbatim}
| |
\end{verbatim}
Extremely high informativeness examples are often foreign language, since they don't contain English stop words:
\begin{small}
\begin{verbatim}
maailmankaikkeuden sinnikkäimmällä valittajahahmolla umayya abu-hannalla on taas
sanottavaa . niin , tiedätte kyllä mistä : suomalaisten ra-sis-mis-ta . 
abu-hannaa haastatellaan päivän helsingin sanomissa ehkä ziljoonannen kerran
tästä yhdestä ja samasta aiheesta . en ymmärrä miksi . abu-hanna on ollut
tällä viikolla suomessa noutamassa global family award -palkintoa ”
avarakatseisuudesta ja monikulttuurisuuden merkittävästä edistämisestä
suomalaisessa yhteiskunnassa ” . avarakatseisuudesta ? ? ? ? ?
en tiedä ketään , jonka katsantokanta on ( julkisen kuvan perusteella ) niin kapea
kuin abu-hannan . hänen toistuvat ” suuri osa suomalaisista on rasisteja ”
-puheenvuoronsa eivät myöskään synnytä minkäänlaista positiivista dialogia tähän
yhteiskuntaan . niistä tykkäävät ja somessa peukuttavat ainoastaan ne ihmiset ,
jotka ovat itsekin sitä mieltä , että suomi on raakalaismaisten rasistien maa .
muissa suomalaisissa ne herättävät kohtuuttomuudessaan ja jankkauksessaan vain
ärtymystä . kuten kaikki tiedämme , abu-hanna asuu nykyään hollannissa . vielä
vuosi sitten kyseinen maa näyttäytyi hänen haastatteluissaan paratiisina . mutta
nyt – ja tämä ei varmasti yllätä ketään –
\end{verbatim}
\end{small}
Examples with informative ratio close to 0.5 are more standard English:
\begin{small}
\begin{verbatim}
the feature ( 2 ) mentioned above . the assumption of $ p $ = 1 might 
be unrealistic in  usual ferromagnetic metals . however , if the exchange
interaction between eu atoms is  accomplished via $ \pi $ -bands of 
c $ _ { 60 } $ as discussed earlier , we can expect a  large spin 
polarization of $ \pi $ -electrons . we can also consider the effect of magnetic
polaron . in magnetic semiconductors such as eu chalcogenides , 
a carrier makes surrounding magnetic moments be polarized via 
exchange interaction and forms a magnetic polaron [ @ kasuya1 ] .
at zero field , magnetic polarons have to move with flipping some 
magnetic moments which are more or less randomly oriented , and their
conduction is suppressed . application of magnetic field aligns spin
directions and carriers become mobile . as a result , negative
magnetoresistance occurs . the negative magnetoresistance above 
$ t_c $ can be attributed to this
\end{verbatim}
\end{small}
